# Supplementary material for: RAVEN: Radar Adaptive Vision Encoders for Efficient Chirp-wise Object Detection and Segmentation
Source: arXiv:2604.04490 source file (2026-04-06)
Supplement: Supplementary file 2 [file supp.tex]

% supp.tex  — standalone supplementary file

\documentclass[10pt,twocolumn,letterpaper]{article}

\usepackage{cvpr}
\input{preamble}

\definecolor{cvprblue}{rgb}{0.21,0.49,0.74}
\usepackage[pagebackref,breaklinks,colorlinks,allcolors=cvprblue]{hyperref}

% Make sure graphicx is loaded in preamble; if not, uncomment:
% \usepackage{graphicx}

\title{RAVEN: Radar Adaptive Vision Encoders for Efficient Chirp-wise Object Detection and Segmentation}

\author{Anuvab Sen\\
Georgia Institute of Technology\\
Atlanta, GA, USA\\
{\tt\small asen74@gatech.edu}
\and
Mir Sayeed Mohammad\\
{\tt\small mirsayeedmohammad@gatech.edu}
\and
Saibal Mukhopadhyay\\
{\tt\small saibal.mukhopadhyay@ece.gatech.edu}
}

\begin{document}
% \maketitlesupplementary
% \setcounter{page}{1}  % start supplement at page 1

\clearpage
\setcounter{page}{1}
\maketitlesupplementary

\section{Rationale}
\label{sec:rationale}
Having the supplementary compiled together with the main paper means that:
\begin{itemize}
\item The supplementary can back-reference sections of the main paper, for example, we can refer to \cref{sec:intro};
\item The main paper can forward reference sub-sections within the supplementary explicitly (e.g. referring to a particular experiment); 
\item When submitted to arXiv, the supplementary will already included at the end of the paper.
\end{itemize}
To split the supplementary pages from the main paper, you can use \href{https://support.apple.com/en-ca/guide/preview/prvw11793/mac#:~:text=Delete%20a%20page%20from%20a,or%20choose%20Edit%20%3E%20Delete).}{Preview (on macOS)}, \href{https://www.adobe.com/acrobat/how-to/delete-pages-from-pdf.html#:~:text=Choose%20%E2%80%9CTools%E2%80%9D%20%3E%20%E2%80%9COrganize,or%20pages%20from%20the%20file.}{Adobe Acrobat} (on all OSs), as well as \href{https://superuser.com/questions/517986/is-it-possible-to-delete-some-pages-of-a-pdf-document}{command line tools}.   % content only, no extra title

{
    \small
    \bibliographystyle{ieeenat_fullname}
    \bibliography{main}
}

\end{document}
